# Supplementary material for: Tunable Luminescence From a Single Free-Base Porphyrin Molecule By Controlled Access to Optically Active States
Source: arXiv:2511.00630 source file (2026-08-18)
Supplement: Supplementary file 1 [file SI.pdf]

# Supporting Information: Accessing Energetically Restricted Optical Transitions in a Single Free-Base Porphyrin Molecule

Eve Ammerman 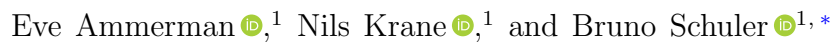<sup>1</sup>, Nils Krane 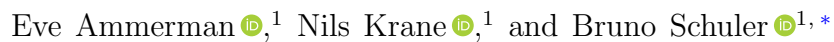<sup>1</sup> and Bruno Schuler 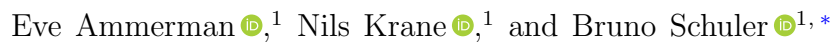<sup>1,\*</sup>

<sup>1</sup>*nanotech@surfaces Laboratory, Empa – Swiss Federal Laboratories  
for Materials Science and Technology, Dübendorf 8600, Switzerland*

(Dated: November 1, 2025)

## CONTENTS

|                                                  |   |
|--------------------------------------------------|---|
| Polaron Model                                    | 2 |
| Theoretical Model for Voltage Dependent Emission | 3 |
| References                                       | 6 |

## POLARON MODEL

The observed  $dI/dV$  peaks of molecules on NaCl are known to be, both, broadened and shifted to higher absolute energy, due to the strong electron-phonon coupling of the underlying salt [1, 2]. To extract the zero-phonon ion resonance energy, we employ a simple polaron model, as described by [3]:

$$S(E_{fi}, Q_{fi}, V) = \frac{1}{2\pi} \text{Re} \left\{ \int dt e^{-ieVt/\hbar} e^{\mathcal{F}(E_{fi}, Q_{fi})} \right\}, \quad \text{with} \quad (\text{S1})$$

$$\mathcal{F}(E_{fi}, Q_{fi}) = -iQ_{fi}E_{fi}t/\hbar + \int_0^\infty d\Omega J(\Omega) e^{-iQ_{fi}\Omega t/\hbar}, \quad (\text{S2})$$

where  $E_{fi}$  is the energy difference between final and initial state and  $Q_{fi}$  a unitless charge number, being +1 or -1 for ionization or electron attachment, respectively. The electron-phonon coupling strength of the NaCl is included in the rectangular function  $J(\Omega)$ , which we assume to have a constant value  $\eta$  between 18 meV and 31 meV and is zero otherwise [3].

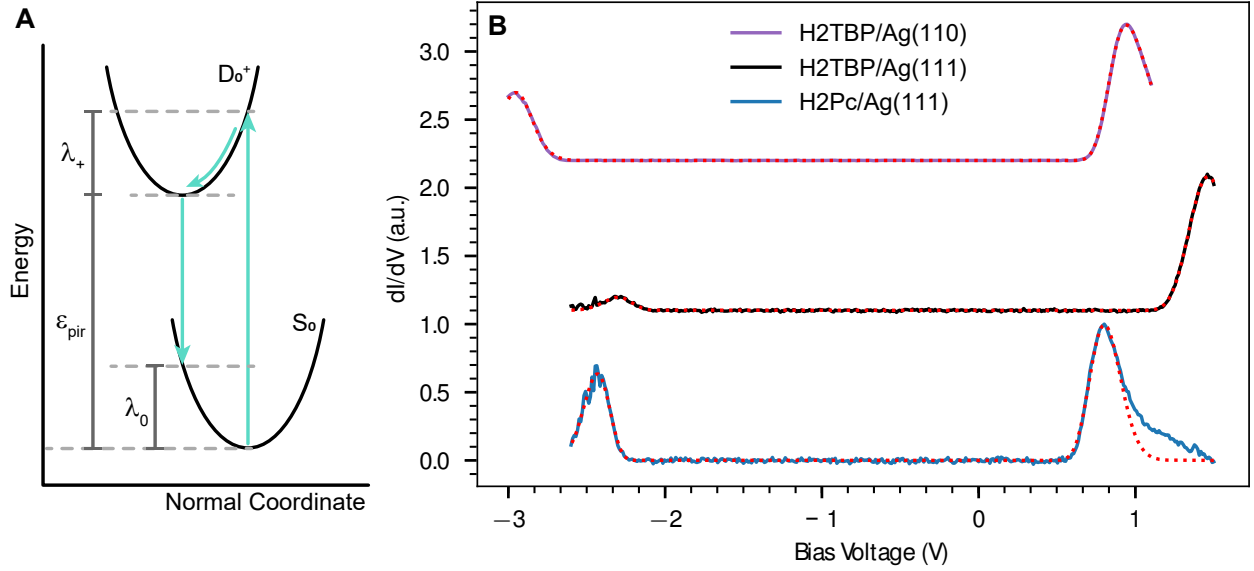

FIG. S1. **Polaron Modeling of  $dI/dV$  measurements** (a) Sketch of the free-energy curves of a neutral and positively charged molecule on NaCl. The relaxation energy for ionization and neutralization are labeled  $\lambda_+$  and  $\lambda_0$ , respectively. (b) Experimental  $dI/dV$  spectra taken on TBP on Ag(110) (purple) and Ag(111) (brown) as well as Pc on Ag(111). Dotted red lines correspond to the model fit w.r.t the corresponding  $dI/dV$  data.

The parameters  $E_{fi}$  and  $\lambda_{\pm}$  are used as fit parameters to fit the polaron model to the  $dI/dV$  spectra. Here,  $E_{fi}$  corresponds to the zero-phonon ion resonance energy (*c.f.*  $\epsilon_{\text{PIR}}$  in

figure S1a) and  $\lambda_{\pm}$  is proportional to the electron-phonon coupling strength  $\eta$ :

$$\lambda = \int_0^{\infty} d\Omega J(\Omega) \hbar \Omega \quad (\text{S3})$$

Fitting was performed with a voltage scale of 0.9 to account for voltage drop across the NaCl. In figure S1 the x-axis of the fit data is rescaled to match the experimental data.

TABLE I. Fitted parameters obtained from polaron model.

| Parameter   | TBP/Ag(111) | TBP/Ag(110) | Pc/Ag(111) |
|-------------|-------------|-------------|------------|
| $E_{D_0^+}$ | 1.812 eV    | 2.248 eV    | 1.984 eV   |
| $\lambda^+$ | 268 meV     | 303 meV     | 216 meV    |
| $E_{D_0^-}$ | 0.832 eV    | 0.543 eV    | 0.422 eV   |
| $\lambda^-$ | 494 meV     | 297 meV     | 311 meV    |

## THEORETICAL MODEL FOR VOLTAGE DEPENDENT EMISSION

The voltage dependence of the emission rate was simulated with a simple rate model, similar to the one discussed in [4]. Here we consider only three states (see Fig. 2a of the main text), namely  $S_0$ ,  $S_1$  and  $D_0^+$ . The energy  $E_{S_1} = 1.915 \text{ eV}$  of the excitonic state is given by the experimentally measured photon energy of the 0-0 line. From the polaron fit, we extracted the the zero-phonon transition energy  $E_{\text{PIR}}$ , which corresponds to  $E_{D_0^+}$

The voltage dependent transition rates between the neutral and the charged state are given by integration of the polaron spectral profile as described in equation S1:

$$\begin{aligned} \Gamma_{S_i \rightarrow D_0^+}(V_{\text{eff}}) &= \frac{2\hat{V}}{h} \int_{V_{\text{eff}}}^{\infty} S(E_{D_0^+} - E_{S_i}, +1, V') dV' \\ \Gamma_{D_0^+ \rightarrow S_i}(V_{\text{eff}}) &= \frac{\hat{V}}{h} \int_{-\infty}^{V_{\text{eff}}} S(E_{S_i} - E_{D_0^+}, -1, V') dV', \end{aligned}$$

with  $\hat{V}$  being the coupling strength of the molecule to tip and surface. The effective bias voltage  $V_{\text{eff}}$  between molecule and corresponding lead is given by the voltage drop  $\alpha \approx 0.1$  and corresponds to  $V_{\text{eff}}^t = (1 - \alpha)V_b$  and  $V_{\text{eff}}^s = -\alpha V_b$  for tip and sample, respectively. The additional factor of two for the singlet to doublet transition yields from multiplicities of the involved states and is given by the Clebsch-Gordan coefficients  $\Upsilon_{fi}$ . As an approximation,

we assume the relaxation energy  $\lambda$  to be the same for all transitions between the positive ion resonance  $D_0^+$  and the charge neutral states  $S_0$  and  $S_1$  ( $\lambda_+^0 = \lambda_0^0 = \lambda_+^1 = \lambda_0^0$ ).

In the bias range of interest we further assume some transition rates to be constant, namely  $\Gamma_{S_0 \rightarrow D_0^+}^s = \Gamma_{D_0^+ \rightarrow S_0}^t = \Gamma_{D_0^+ \rightarrow S_1}^t = 0$  as well as  $\Gamma_{S_0^+ \rightarrow S_0}^s = \hat{V}_t/h$ . We estimated the coupling to the substrate to be  $\hat{V}_s = 4 \text{ meV}$  and used the coupling to the tip  $\hat{V}_t$  as a fitting parameter. For the radiative emission  $\Gamma_{S_1 \rightarrow S_0}^{\text{ph}} = \hat{V}_{\text{ph}}/h$  the lifetime was estimated from the width of the emission peak to be in the order of  $\hat{V}_{\text{ph}} = 1 \text{ meV}$ .

In this simplified model, we do not directly include the  $T_1$  triplet state and experimentally there is no indication of triplet pumping [4]. However, the presence of the triplet state causes an increase in the dark current as it opens another channel to neutralize the molecule via sample from the  $D_0^+$  state into  $T_1$  and then decay non-radiatively back into the ground state  $S_0$ . To capture this effect, the transition rate  $\Gamma_{D_0^+ \rightarrow S_0}^s$  is multiplied with a factor of 2.5, consisting of the Clebsh-Gordan coefficients  $\Upsilon_{D_0^+ \rightarrow S_0} = 1$  and  $\Upsilon_{D_0^+ \rightarrow T_1} = 1.5$ .

The occupation probability  $N_i$  of the three considered states  $S_0$ ,  $S_1$  and  $D_0^+$  is solved using a differential rate equation for the steady state condition  $0 = \sum_j \Gamma_{j \rightarrow i}(V_b)N_j - \Gamma_{i \rightarrow j}(V_b)N_i$  at given bias voltage  $V_b$ . The total current is then defined by  $I_e(V) = e^-(\Gamma_{S_0 \rightarrow D_0^+}^t N_{S_0} - \Gamma_{S_1 \rightarrow D_0^+}^t N_{S_1})$  and the emitted light intensity by  $I_{\text{ph}}(V) = A\Gamma_{S_1 \rightarrow S_0}^{\text{ph}} N_{S_1}$ , with  $A < 1$  representing the detection efficiency.

The modeled current and light intensity are fitted to experiment, using tip coupling  $\hat{V}_t$ , voltage drop  $\alpha$  and photon detection efficiency  $A$  as fitting parameter. For the normalized STML intensity we added an additional background current  $I_{\text{bg}} = 150 \text{ fA}$ , corresponding to tunneling directly into the substrate:  $I_{\text{ph}}/(I_e + I_{\text{bg}})$ . The resulting fits are displayed in Figure S2 and the corresponding parameter listed in table II.

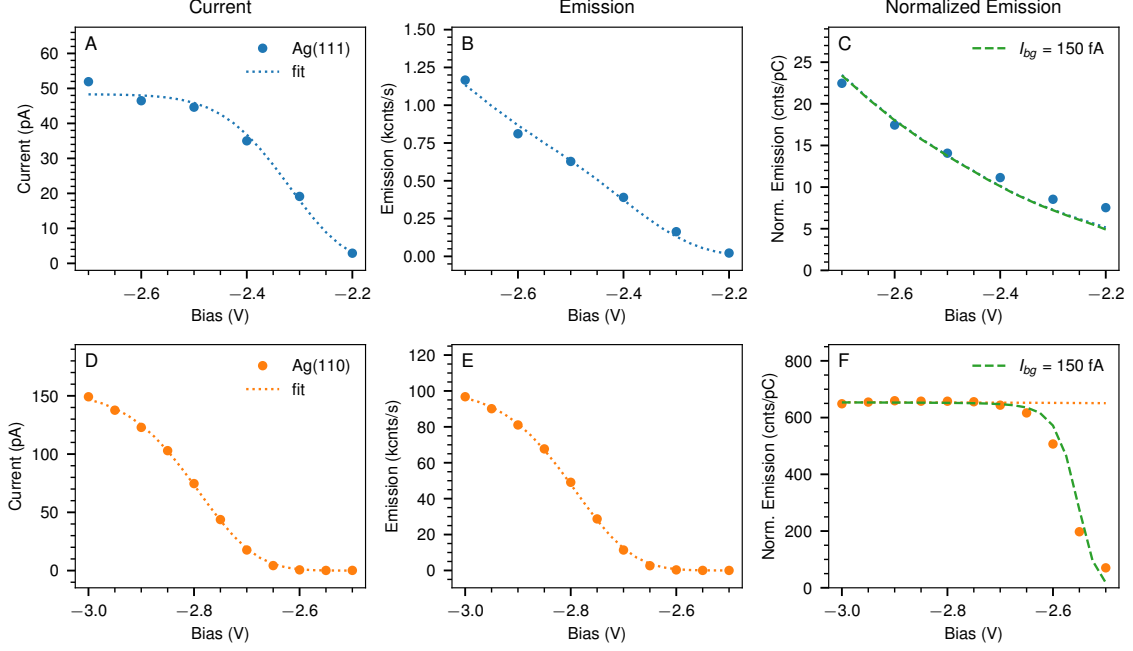

FIG. S2. **Modeling of STML data.** Bias dependent current and STML intensity of the 0-0 emission from H<sub>2</sub>TBP on NaCl/Ag(111) (A-C) and NaCl/Ag(110) (D-F).

TABLE II. **Parameters used to model the STML intensity.**  $E_{D_0^+}$  and  $\lambda^+$  were obtained from the polaron model.  $A$ ,  $\alpha$  and  $\hat{V}_t$  were used as fitting parameters for the rate equation model.

| Parameter   | TBP/Ag(111)          | TBP/Ag(110)          |
|-------------|----------------------|----------------------|
| $E_{S_0}$   | 0 eV                 |                      |
| $E_{S_1}$   | 1.915 eV             |                      |
| $E_{D_0^+}$ | 1.812 eV             | 2.248 eV             |
| $\lambda^+$ | 268 meV              | 303 meV              |
| $A$         | $1.27 \cdot 10^{-4}$ | $3.70 \cdot 10^{-4}$ |
| $\alpha$    | 10.2%                | 9.0%                 |
| $\hat{V}_t$ | 0.7 $\mu$ eV         | 2.7 $\mu$ eV         |
| $\hat{V}_s$ | 4 meV                |                      |

---

\* [bruno.schuler@empa.ch](mailto:bruno.schuler@empa.ch)

- [1] J. Repp, G. Meyer, S. Paavilainen, F. E. Olsson, and M. Persson, [Phys. Rev. Lett. \*\*95\*\*, 225503 \(2005\)](#).
- [2] S. Fatayer, B. Schuler, W. Steurer, I. Scivetti, J. Repp, L. Gross, M. Persson, and G. Meyer, [Nat. Nanotechnol. \*\*13\*\*, 376 \(2018\)](#).
- [3] K. Vasilev, S. Canola, F. Scheurer, A. Boeglin, F. Lotthammer, F. Chérioux, T. Neuman, and G. Schull, [ACS Nano \*\*18\*\*, 28052 \(2024\)](#).
- [4] K. Kaiser, A. Rosławska, M. Romeo, F. Scheurer, T. c. v. Neuman, and G. Schull, [Phys. Rev. X \*\*15\*\*, 021072 \(2025\)](#).
